# Supplementary material for: Exploiting Variational Domain-Invariant User Embedding for Partially Overlapped Cross Domain Recommendation
Source: arXiv:2205.06440 source file (2022-05-27)
Supplement: Supplementary file 1 [file appendix.tex]

% \appendix

% \section{Datasets and Tasks} 
% %
% We conduct extensive experiments on two popularly used real-world datasets, i.e., \textit{Douban} and \textit{Amazon}, for evaluating our models on PUCDR tasks \cite{dtcdr,gadtcdr,amazon}.
% %
% First, the \textbf{Douban} dataset \cite{dtcdr,gadtcdr} has two domains, i.e., Book and Movie, with user-item ratings. 
% %
% Second, the \textbf{Amazon} dataset \cite{catn,amazon} has four domains, i.e., Movies and TV (Movie), Books (Book), CDs and Vinyl (Music), and Clothes (Clothes).
% %
% The detailed statistics of these datasets after pre-process will be shown in Table 3.



% \section{Analysis} 
% %
% \nosection{Effect of hyper-parameters}
% %
% we conduct the experiments by varying $\lambda_{VL}$ and $\lambda_{VG}$ in $\{0.1,0.3,0.5,0.7,1,3,5,10\}$ and report the results in Fig.~6(a)-(b).
% %
% When $\lambda_{VL},\lambda_{VG} \rightarrow 0$, the alignment loss cannot produce the positive effect.
% %
% When $\lambda_{VL}$ and $\lambda_{VG}$ become too large, the alignment loss will suppress the rating reconstruction loss, which also decreases the recommendation results.
% %
% Empirically, we choose $\lambda_{VL} = 0.7$ and $\lambda_{VG} = 1.0$.

% \begin{figure} 
%     \centering
%         \subfigure[Effect of $\lambda_{VL}$]{
%     \begin{minipage}[t]{0.47\linewidth} %0.23为minipage的宽度，可以调节子图间的距离
%     \includegraphics[width=4.2cm]{pic/w3.pdf}
%     \end{minipage}
% }
%         \subfigure[Effect of $\lambda_{VG}$]{
%     \begin{minipage}[t]{0.47\linewidth} %0.23为minipage的宽度，可以调节子图间的距离
%     \includegraphics[width=4.2cm]{pic/w4.pdf}
%     \end{minipage}
% }
% \vspace{-0.3cm}
% 	  \caption{(a)-(b) show the effect of  $\lambda_{VL}$ and $\lambda_{VG}$ on model performance. }
% 	  \label{fig1:param}
% \vspace{-0.3cm}
% \end{figure}
